# Supplementary material for: Outlier-robust Kalman Filtering through Generalised Bayes
Source: arXiv:2405.05646 source file (2024-05-28)
Supplement: Supplementary file 1 [file ensemble-dep.tex]

\clearpage
\section{Likelihood-weighted ensemble}

\mj{This section is reinstated temporarily, so that comments in the previous subsection can reference its contents.}

We propose a weighted version of EnKF based on our WLF, summarized in \cref{algo:wEnKF-update,algo:wEnKF-weight,algo:wEnKF-sample,algo:wEnKF-gain,algo:wEnKF-update-particles,algo:wEnKF-particle-specific-wt}. The weighted EnKF modifies equation \eqref{eq:EnKF-sampling} to sample predictions from the same weighted loglikelihood that the WLF uses for inference. 
We list here several forms of this sampling rule:
for the general case with a scalar weight $W_t(\vy_{1:t})$ as in \cref{eq:weighted-loglikelihood}
the log-likelihood is given by
\begin{equation}
\log p\left(\hat{\vy}_{t\vert t-1}^{\left(i\right)}\vert\hat{\vtheta}_{t\vert t-1}^{\left(i\right)}\right) = W_{t}^{2}(\vy_{1:t})\log p\left(\vy_t\vert \hat{\vtheta}_{t\vert t-1}^{\left(i\right)}\right) + C,
\label{eq:wEnKF-sampling-gen}
\end{equation}
for a scalar weight and Gaussian likelihood as in \cref{eq:weighted-gaussian-loglikelihood}:
\begin{align}
    p\left(\hat{\vy}_{t|t-1}^{(i)}|\hat{\vtheta}_{t|t-1}^{(i)}\right)=\gauss\left(\vy_t|h_t\left(\hat{\vtheta}_{t|t-1}^{(i)}\right),W_t^{-2}(\vy_{1:t})\vR_t\right),
    \label{eq:wEnKF-sampling-gauss}
\end{align}
for dimension-specific weights and general conditionally independent likelihood as in \cref{eq:weighted-independent-loglikelihood}:
\begin{align}
    \log p\left(\hat{\vy}_{t|t-1}^{(i)}|\hat{\vtheta}_{t|t-1}^{(i)}\right)= \sum_j w^2_{t,j} \log p\left(y_{t,j}|\hat{\vtheta}_{t|t-1}^{(i)}\right),
    \label{eq:wEnKF-sampling-dim-indep}
\end{align}
and for dimension-specific weights and Gaussian likelihood as in \cref{eq:dim-weighted-gaussian-likelihood}:
\begin{align}
    p\left(\hat{\vy}_{t|t-1}^{(i)}|\hat{\vtheta}_{t|t-1}^{(i)}\right)
    =\gauss\left(\vy_t|h_t\left(\hat{\vtheta}_{t|t-1}^{(i)}\right),\bar{\vR}_t\right).
    \label{eq:wEnKF-sampling-Rtilde}
\end{align}

The weighted EnKF converges to the WLF in the linear-Gaussian limit, by the same argument for the vanilla EnKF and EKF in \cref{eq:EnKF-cross_cov-lin_gauss_limit,eq:EnKF-var-lin_gauss_limit,eq:EnKF-gain-lin_Gauss_limit,eq:EnKF-gain-lin_Gauss_limit-b,eq:EnKF-mean-update-lin_gauss_limit,eq:EnKF-cov-update-lin_gauss_limit}. Specifically, the sampling scheme in \cref{eq:wEnKF-sampling-Rtilde} converges to
\begin{align}
\bar{\vK}_t &=
    \vSigma_{t\vert t-1}\vH_{t}^{\top}\left(\vH_{t}\vSigma_{t\vert t-1}\vH_{t}^{\top}+\bar{\vR}_{t}\right)^{-1}\\
\vmu_{t}  &=
    \vmu_{t\vert t-1}+ \bar{\vK}_{t}\left(\vy_{t}-\vH_{t}\vmu_{t\vert t-1}\right)\\
\vSigma_{t} &=
    \vSigma_{t\vert t-1}-\bar{\vK}_{t}\vH_{t}\vSigma_{t\vert t-1}
    \label{eq:wEnKF-cov-update-lin_gauss_limit}
\end{align}
which matches the WLF update in \cref{eq:WLF-dim-cov-update,eq:WLF-dim-mean-update,eq:WLF-dim-gain}
and hence also the update step shown in Algorithm \ref{algo:wlf-step}.

When $W_{t}(\vy_{1:t})=0$ as happens for the MD weighting,
the method described here becomes degenerate but corresponds to a limit in which
the $\hat{\vy}_{t\vert t-1}^{\left(i\right)}$ have infinite variance and hence $\bar{\vK}_{t}=\bm{0}$.
Thus in practice when $W_t(\vy_{1:t})=0$, we skip the sampling and simply do not update the particles.
When using dimension-specific weights and $w_{t,j}=0$ for one or more observation dimensions, the ensemble update uses only the observations with positive weights.
More precisely, define the mask
$\vm_t=\{j:w_{t,j}>0\}$
and use \cref{eq:wEnKF-sampling-gen,eq:wEnKF-sampling-gauss,eq:wEnKF-sampling-dim-indep,eq:EnKF-sampling-Rtilde} to sample only 
$\hat{\vy}_{t|t-1,\,\vm_t}$.
Then the ensemble cross-covariance and variance in \cref{eq:enkf-gain-matrix} respectively have dimension $\nparams\times|\vm_t|$ and $|\vm_t|\times|\vm_t|$ so $\bar{\vK}$ has dimension $\nparams\times|\vm_t|$, and we modify the particle update in \cref{eq:EnKF-update} to use only the errors on observations in $\vm_t$:
\begin{equation}
\hat{\vtheta}_{t}^{\left(i\right)}=
\hat{\vtheta}_{t\vert t-1}^{\left(i\right)}+\bar{\vK}_{t}\left(\vy_{t,\vm_t}-\hat{\vy}_{t\vert t-1,\,\vm_t}^{(i)}\right).
\end{equation}

\begin{algorithm}[hbt]
\begin{algorithmic}[1]
\STATE \textbf{Def} ${\rm ensemble\_update}\left(\left(\hat{\vtheta}_{t\vert t-1}^{\left(i\right)}\right)_{i\in\left[N\right]},h_{t}\left(\cdot\right),\vy_{t},p_{\vy_{t}\vert\vh_{t}}\left(\cdot\vert\cdot\right),W_{t}\left(\cdot,\cdot\right)\right)$:
    \begin{ALC@g}
    \STATE \textbf{For} $i\in\left[N\right]$:
        $\hat{\vh}_{t\vert t-1}^{\left(i\right)}=h_{t}\left(\hat{\vtheta}_{t\vert t-1}^{\left(i\right)}\right)$
    \STATE $\vw_{t}={\rm ensemble\_weight}\left(\vy_{t},\left(\hat{\vh}_{t\vert t-1}^{\left(i\right)}\right)_{i\in\left[N\right]},p_{\vy_{t}\vert\vh_{t}}\left(\cdot\vert\cdot\right),W_{t}\left(\cdot,\cdot\right)\right)$
    \STATE $\left(\hat{\vy}_{t\vert t-1}^{\left(i\right)}\right)_{i\in\left[N\right]}={\rm sample\_predictions}\left(\left(\hat{\vh}_{t\vert t-1}^{\left(i\right)}\right)_{i\in\left[N\right]},\vw_{t},p_{\vy_{t}\vert\vh_{t}}\left(\cdot\vert\cdot\right)\right)$
    \STATE $\bar{\vK}_{t}={\rm gain}\left(\left(\hat{\vtheta}_{t\vert t-1}^{\left(i\right)}\right)_{i\in\left[N\right]},\left(\hat{\vy}_{t\vert t-1}^{\left(i\right)}\right)_{i\in\left[N\right]},I\left\{ \vw_{t}>0\right\} \right)$
    \STATE $\left(\hat{\vtheta}_{t}^{\left(i\right)}\right)_{i\in\left[N\right]}={\rm update\_particles}\left(\left(\hat{\vtheta}_{t\vert t-1}^{\left(i\right)}\right)_{i\in\left[N\right]},\left(\hat{\vy}_{t\vert t-1}^{\left(i\right)}\right)_{i\in\left[N\right]},\vy_{t},\bar{\vK}_{t}\right)$
    \STATE \textbf{Return} $\left(\hat{\vtheta}_{t}^{\left(i\right)}\right)_{i\in\left[N\right]}$
    \end{ALC@g}
\end{algorithmic}
\caption{
    wEnKF update step
}
\label{algo:wEnKF-update}
\end{algorithm}

\begin{algorithm}[htb]
\begin{algorithmic}[1]
\STATE \textbf{Def} ${\rm ensemble\_weight}\left(\vy,\left(\hat{\vh}^{\left(i\right)}\right)_{i\in\left[N\right]},p\left(\cdot\vert\cdot\right),W\left(\cdot,\cdot\right)\right)$:
    \begin{ALC@g}
    \STATE \textbf{For} $i\in[N]$: 
        $\bar{\vy}^{\left(i\right)}=\expectQ{\vy}{\vy\sim p\left(\cdot\vert\hat{\vh}^{\left(i\right)}\right)}$
        // for Gaussian likelihood this is just $\bar{\vy}^{\left(i\right)}=\hat{\vh}^{\left(i\right)}$
    \STATE \textbf{Case}: Mean prediction method (``hard weights'')
        \begin{ALC@g}
        \STATE $\bar{\vy}=\frac{1}{N}\sum_{i}\bar{\vy}^{\left(i\right)}$
        \STATE $\vw=W\left(\vy,\bar{\vy}\right)$
        \end{ALC@g}
    \STATE \textbf{Case}: Mean weight method (``soft weights'')
        \begin{ALC@g}
        \STATE \textbf{For} $i\in\left[N\right]$: $\vw^{\left(i\right)}=W\left(\vy,\bar{\vy}^{\left(i\right)}\right)$
        \STATE $\vw=\frac{1}{N}\sum_{i}\vw^{\left(i\right)}$
        \end{ALC@g}
    \STATE \textbf{Return} $\vw$
    \end{ALC@g}
\end{algorithmic}
\caption{
    wEnKF weight calculation
}
\label{algo:wEnKF-weight}
\end{algorithm}

\begin{algorithm}[htb]
\begin{algorithmic}[1]
\STATE \textbf{Def} ${\rm sample\_predictions}\left(\left(\hat{\vh}^{\left(i\right)}\right)_{i\in\left[N\right]},\vw,p\left(\cdot\vert\cdot\right)\right)$:
    \begin{ALC@g}
    \STATE \textbf{Case}: Conditionally independent likelihood $p\left(\vy\vert\vh\right)=\prod_{j}p_{j}\left(y_{j}\vert\vh\right)$:
        \begin{ALC@g}
        \STATE \textbf{For} $j$ with $w_{j}>0$:
            \begin{ALC@g}
            \STATE \textbf{For} $i\in\left[N\right]$: $\hat{y}_{j}^{\left(i\right)}\sim p_{j}\left(y_{j}\vert\hat{\vh}^{\left(i\right)}\right)^{w_{j}^2}$
            \end{ALC@g}
        \STATE \textbf{For} $j$ with $w_{j}=0$:
            \begin{ALC@g}
            \STATE \textbf{For} {$i\in\left[N\right]$}: $\hat{y}_{j}^{\left(i\right)}=0$
            \end{ALC@g}
        \end{ALC@g}
    \STATE \textbf{Case}: Nondiagonal Gaussian likelihood $p\left(\cdot\vert\vh\right)=\gauss\left(\cdot\vert\vh,\vR\right)$
        \begin{ALC@g}
        \STATE $\vw_{\left\{ \vw=0\right\} }=\bm{1}$ // arbitrary; these samples will be ignored
        \STATE $\bar{\vR}=\Diag\left(\vw\right)^{-1}\vR\Diag\left(\vw\right)^{-1}$
        \STATE \textbf{For} $i\in\left[N\right]$: $\hat{\vy}^{\left(i\right)}\sim\gauss\left(\hat{\vh}^{\left(i\right)},\bar{\vR}\right)$
        \end{ALC@g}
    \STATE \textbf{Return} $\left(\hat{\vy}^{\left(i\right)}\right)_{i\in\left[N\right]}$
    \end{ALC@g}
\end{algorithmic}
\caption{
    wEnKF prediction sampling
}
\label{algo:wEnKF-sample}
\end{algorithm}

\begin{algorithm}[htb]
\begin{algorithmic}[1]
\STATE \textbf{Def} ${\rm Gain}\left(\left(\hat{\vtheta}^{\left(i\right)}\right)_{i\in\left[N\right]},\left(\hat{\vy}^{\left(i\right)}\right)_{i\in\left[N\right]},\text{bool: }\vm\right)$:
    \begin{ALC@g}
    \STATE $\vM={\rm cov}_{i}\left[\hat{\vtheta}^{\left(i\right)},\hat{\vy}^{\left(i\right)}\right]$
    \STATE $\vS=\varQ{\hat{\vy}^{\left(i\right)}}{i}$
    \STATE \textbf{For} $j$ with $\neg m_{j}$:
        \begin{ALC@g}
        \STATE $S_{j,j}=1$
        \STATE \textbf{For} $j'\ne j$: $S_{j,j'}=S_{j',j}=0$ // can skip (already true) in case of conditionally independent likelihood
        \end{ALC@g}
    \STATE $\bar{\vK}=\vM\Diag\left(\vm\right)\vS^{-1}\Diag\left(\vm\right)$ // Jax-friendly implementation of $\bar{\vK}\ve=\vM_{\cdot,\vm}\left(\vS_{\vm,\vm}\right)^{-1}\ve_{\vm}$
    \STATE \textbf{Return} $\bar{\vK}$
    \end{ALC@g}
\end{algorithmic}
\caption{
    wEnKF gain calculation
}
\label{algo:wEnKF-gain}
\end{algorithm}

\begin{algorithm}[htb]
\begin{algorithmic}[1]
\STATE \textbf{Def} ${\rm update\_particles}\left(\left(\hat{\vtheta}_{t\vert t-1}^{\left(i\right)}\right)_{i\in\left[N\right]},\left(\hat{\vy}^{\left(i\right)}\right)_{i\in\left[N\right]},\vy,\bar{\vK}\right)$:
    \begin{ALC@g}
    \STATE \textbf{For} $i\in\left[N\right]$:
        \begin{ALC@g}
        \STATE $\ve^{\left(i\right)}=\vy-\hat{\vy}^{\left(i\right)}$
        \STATE $\hat{\vtheta}_{t}^{\left(i\right)}=\hat{\vtheta}_{t\vert t-1}^{\left(i\right)}+\bar{\vK}\ve^{\left(i\right)}$
        \end{ALC@g}
    \STATE \textbf{Return} $\left(\hat{\vtheta}_{t}^{\left(i\right)}\right)_{i\in\left[N\right]}$
    \end{ALC@g}
\end{algorithmic}
\caption{
    wEnKF particle update
}
\label{algo:wEnKF-update-particles}
\end{algorithm}

\begin{algorithm}[ht]
\begin{algorithmic}[1]
    \STATE ${\rm ensemble\_weight}$: Return $\left(\vw^{\left(i\right)}\right)_{i\in\left[N\right]}$
    \STATE ${\rm sample\_predictions}$: Use $\vw^{\left(i\right)}$ in place of $\vw$
    \STATE ${\rm update\_particles}$: Weight each particle's error by $\vw^{\left(i\right)}$, normalized per dimension
        \begin{ALC@g}
        \STATE $\bar{w}_{j}^{\left(i\right)}=\frac{w_{j}^{\left(i\right)}}{\sum_{i'}\bar{w}_{j}^{\left(i'\right)}}$
        \STATE $\hat{\vtheta}_{t}^{\left(i\right)}=\hat{\vtheta}_{t\vert t-1}^{\left(i\right)}+\bar{\vK}_{t}\Diag\left(\bar{\vw}^{\left(i\right)}\right)\ve_{t}^{\left(i\right)}$
        \end{ALC@g}
\end{algorithmic}
\caption{
    wEnKF variations for particle-specific weighting in sampling and/or updating
}
\label{algo:wEnKF-particle-specific-wt}
\end{algorithm}
